# Supplementary material for: Colossal pressure-induced softening in scandium fluoride
Source: arXiv:2003.13475 source file (2020-03-30)
Supplement: Supplementary file 1 [file ScF3_softening_supplementary.pdf]

# Colossal pressure-induced softening in scandium fluoride: Supplementary materials

Zhongsheng Wei,[1*] Lei Tan,[1*] Guanqun Cai,[1*] Anthony E Phillips,[1]
Ivan da Silva,[2] Mark G Kibble,[2] Martin T Dove[3,4,1‡]

[1]School of Physics & Astronomy, Queen Mary University of London,
Mile End Road, London, E1 4ES, United Kingdom
[2]ISIS Neutron and Muon Facility, Rutherford Appleton Laboratory,
Harwell Campus, Didcot, Oxfordshire, OX11 0QX, United Kingdom
[3]College of Computer Science, Sichuan University, Chengdu,
Sichuan 610065, People's Republic of China
[3]Department of Physics, School of Sciences, Wuhan University of Technology,
205 Luoshi Road, Hongshan district, Wuhan, Hubei 430070, People's Republic of China
[*]Joint and equal first authors, no significance to the order.
[‡]To whom correspondence should be addressed; E-mail: martin.dove@icloud.com.

## S1 Notes on the crystal structure of $ScF_3$

The crystal structure has cubic symmetry, space group $Pm\overline{3}m$ (number 221). We describe the asymmetric unit with Sc with fractional coordinates $(0, 0, 0)$ and F with fractionalal coordinates $(0, 0, \frac{1}{2})$. In this setting, the mean-square displacements of the atoms are subject to the symmetry constraints $U_{11}(\mathrm{Sc}) = U_{22}(\mathrm{Sc}) = U_{33}(\mathrm{Sc})$, where $U_{11} = \langle u_x^2 \rangle$ etc., and $U_{11}(\mathrm{F}) = U_{22}(\mathrm{F}) \neq U_{33}(\mathrm{F})$. We find here that $U_{11}(\mathrm{F}) > U_{33}(\mathrm{F})$.

# S2 Molecular dynamics simulations

## S2.1 The model

Our model has three components, in line with the simple one-dimensional model studied previously. We first have a potential energy function to represent the Sc–F bond, and for this we choose the anharmonic Morse potential:

$$E(r) = D\left(\exp(-2\alpha(r - r_0)) - 2\exp(-\alpha(r - r_0))\right) \tag{S1}$$

where $r$ is the instantaneous atomic separation, $r_0$ is the equilibrium separation, $D$ is the depth of the energy well, and $\alpha$ represents the curvature of the energy function. This function has force constant $\partial^2 E/\partial r^2 = 2\alpha^2 D$ at $r = r_0$. To this we add two terms based on bond angles, The first is a relatively stiff term for the F–Sc–F right angle bond angle $\theta$, of the form

$$E(\theta) = \frac{1}{2}k\cos^2\theta = \frac{1}{4}k(1 + \cos 2\theta) \tag{S2}$$

where $k$ is the force constant, and the function has minimum value of zero when $\theta = 90°$. The second bond angle term arises from the linear Sc–F–Sc bond angle $\phi$, and has the form

$$E(\phi) = A(1 + \cos\phi) \tag{S3}$$

where $A$ is the force constant, and the function has minimum value of zero when $\phi = 180°$. Both functions are anharmonic in angle, and of course the angles themselves are anharmonic functions of atomic displacements.

Starting values of the force constants $D$, $\alpha$, $k$ and $A$ were estimated by calculating the phonon dispersion curves and comparing with those calculated by DFT (*1*) (the value of $r_0$ was set as half the unit cell length). Calculations were performed using the GULP code (*2, 3*). The calculated dispersion curves are shown in Figure S1. In this diagram we colour the dispersion curves according to the value of the mode Grüneisen parameter following methods we have

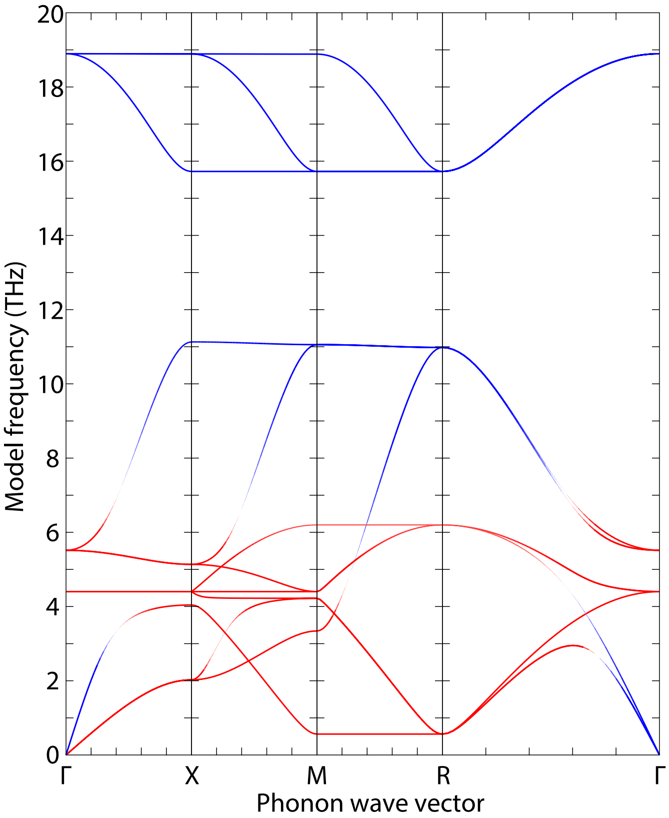


Figure S1: Calculated dispersion curves of $ScF_3$ based on the model indicated in equations S1–S3. The curves are coloured red if they have negative values of the mode Grüneisen parameter, and blue if they have positive values, with the intensity of the colour reflecting the modulus of the value mode Grüneisen parameter up to some saturation value. In this calculation $D =$ 2.0 eV, $r_0 = 2.0125$ Å, $\alpha = 1.55$ Å$^{-1}$, $k = 1.5$ eV, and $A = 0.025$ eV.

described previously (*4*). What is interesting is the extent to which the simple model reflects the DFT dispersion curves, both in overall shape and in the distribution of values, including sign, of mode Grüneisen parameters. The main peculiarity of the model is that the elastic constant $C_{12} = 0$, far from the normal Cauchy relationship for cubic materials with central forces of $C_{12} = C_{44}$. This has little effect on the physical properties.

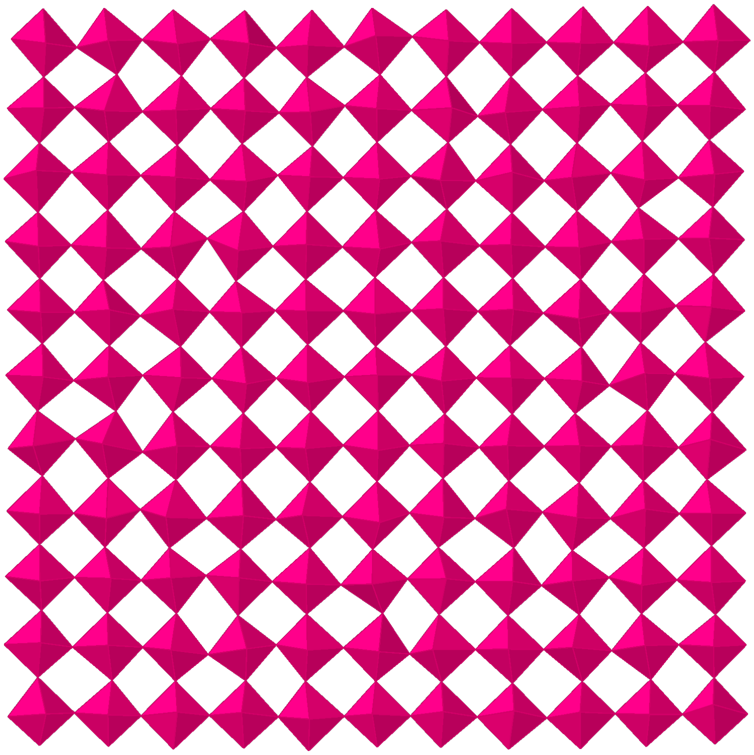

Figure S2: One layer of a single configuration of $ScF_3$ from simulation performed at 1000 K and ambient pressure.

## S2.2 Details of the simulations

The model was studied primarily using the molecular dynamics method, with calculations carried out using the DL_POLY code (*5*). In each case we used a time step of 0.005 ps. For simulations as a function of pressure we used the constant-stress constant-temperature ensemble using the Nosé–Hoover algorithm, and for other analyses we used the microcanonical constant-volume constant-energy ensemble. The simulations were performed with 12 unit cells in each direction (total 6912 atoms). An example of an equilibrated atomic configuration for 1000 K and ambient pressure is shown in Figure S2.

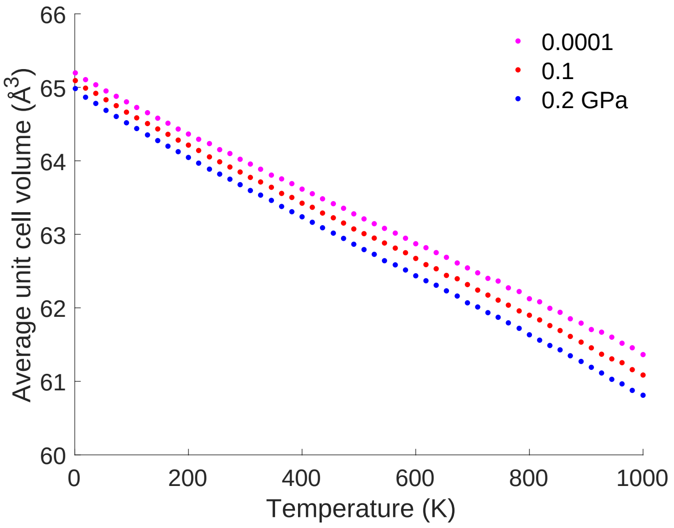


Figure S3: Variation of the unit cell volume with temperature for three pressures calculated by molecular dynamics simulation using the model described in the text.

## S2.3 Pertinent results

The temperature dependence of the volume of the unit cell at ambient pressure and elevated pressures is shown in Figure S3. The model predicts the existence of negative thermal expansion as expected, and the coefficient of thermal expansion becomes more negative on increased pressure as expected by the relationship (*6*)

$$\left(\frac{\partial \alpha_V}{\partial P}\right)_T = \frac{1}{B^2}\left(\frac{\partial B}{\partial T}\right)_P \tag{S4}$$

One difference from experiment is that the negative thermal expansion at ambient pressure continues to a temperature of 1000 K, although in experiment the coefficient of thermal expansion rises to zero at a temperature just above 1000 K (*7*). Given the intended simplicity of our model, and the fact that here we work only at temperatures below 325 K, this difference is not significant.

The temperature-dependence of the atomic displacement parameters $U_{11}$ for Sc and $U_{11}$ and $U_{33}$ for F at ambient pressure from simulation are shown in Figure S4. It is seen that all

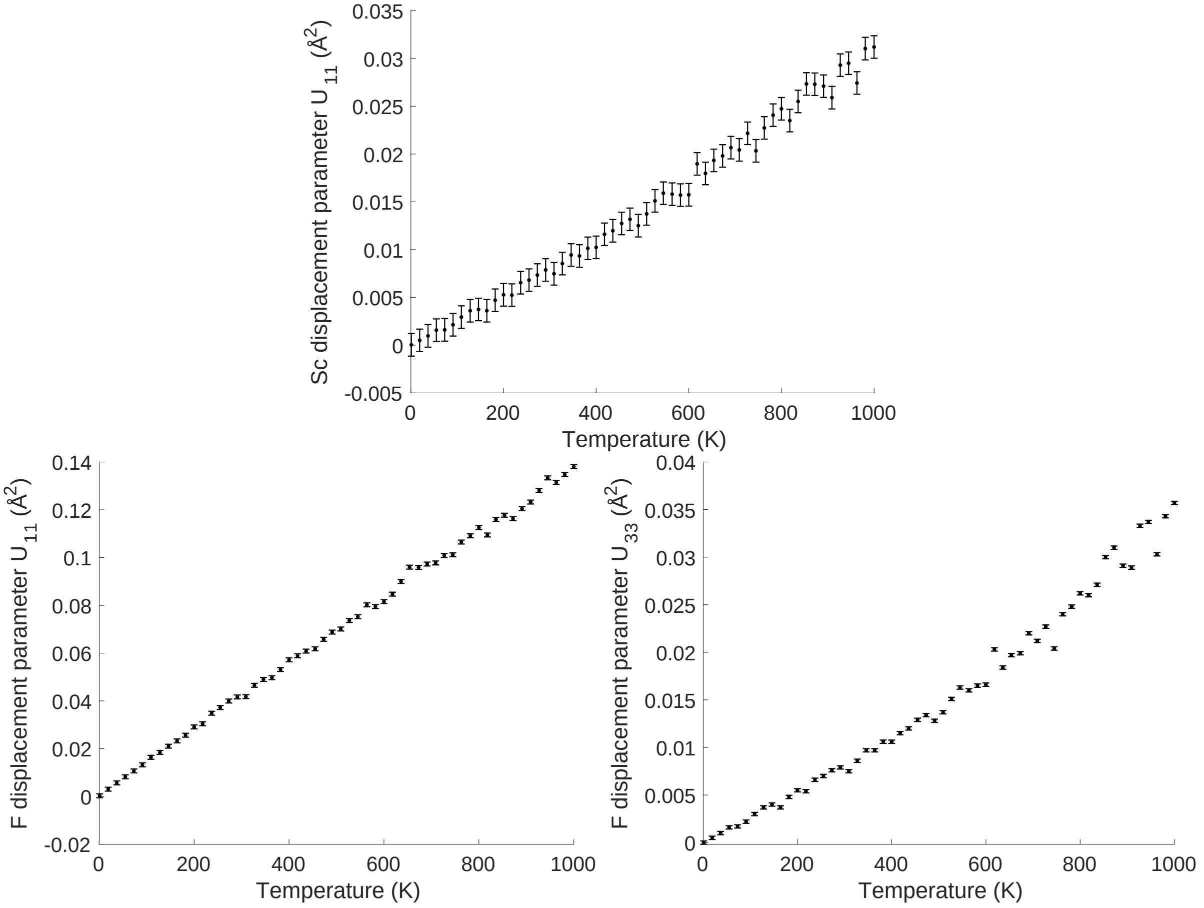


Figure S4: Variation of the Sc $U_{11}$ and F $U_{11}$ and $U_{33}$ with temperature at a small number of pressures calculated by molecular dynamics simulation using the model described in the text.

three vary linearly with temperature as expected, and that for F $U_{11} > U_{33}$ consistent with our understanding of the dynamics of $ScF_3$.

The pressure dependence of the atomic displacement parameters for a few temperatures from simulation are shown in Figure S5. The isotropic $U_{11}$ for Sc and the longitudinal $U_{11}$ for F are effectively constant for all pressures, but the value of $U_{33}$ for F increases with pressure. As discussed in the main text, this is uncommon but consistent with our understanding of pressure-induced softening in $ScF_3$.

# S3 Experimental methods

## S3.1 Neutron diffraction methods

Neutron powder diffraction measurements were performed on the GEM diffractometer at ISIS. A powdered sample of $ScF_3$, obtained commercially from Sigma-Aldrich, was contained within a Ti-Zr alloy pressure cell, which produces a featureless background in the diffraction pattern. The pressure cell was contained within a closed-cycle refrigerator, allowing us to control both temperature and pressure. Hydrostatic pressure applied to the sample was generated by an external pressure intensifier unit to an accuracy of 1 bar. The sample temperature was controlled over a temperature range of 4 to 325 K.

## S3.2 Rietveld refinements

The diffraction data were processed to form a set of data for Rietveld refinement using the MANTID software (). Rietveld refinement was performed using the GSAS II program (*8*). The background signal was modelled using a Chebychev polynomial with 6 coefficients. Lineshape parameters were refined once, and thereafter were held fixed for each separate refinement. As a result, thereafter we refined only the lattice parameter and the three atomic displacement parameters for each sample. The quality of the Rietveld refinement is shown in Figure S6. No account was taken of the attenuation of the beam by sample and pressure system in the refinement. As a result, the values of some atomic displacement parameters are negative.

## S3.3 Pertinent results

The temperature dependence of the atomic displacement parameters $U_{11}$ for Sc and $U_{11}$ and $U_{22}$ for F at ambient pressure refinement from the experimental data are shown in Figure S7. All three vary linearly with temperature as expected, and again we find for F $U_{22} > U_{11}$. The negative values are consistent with not including the effects of beam attenuation in the refinement

process, which at this point could be taken into account by a positive constant shift of all values.

The pressure dependence of the atomic displacements parameters $U_{11}$ for Sc and the longitudinal $U_{33}$ for F for a few temperatures as obtained by Rietveld refinement are shown in Figure S8. The corresponding data for F $U_{11}$ are given in the main text, Figure 6.

# References


1. C. W. Li, *et al.*, *Physical Review Letters* **107**, 195504 (2011).
2. J. D. Gale, A. L. Rohl, *Molecular Simulation* **29**, 291 (2003).
3. J. D. Gale, *Journal of the Chemical Society, Faraday Transactions* **93**, 629 (1997).
4. L. H. N. Rimmer, M. T. Dove, *Journal of Physics: Condensed Matter* **27**, 185401 (2015).
5. I. T. Todorov, W. Smith, K. Trachenko, M. T. Dove, *Journal of Materials Chemistry* **16**, 1911 (2006).
6. M. T. Dove, H. Fang, *Reports on Progress in Physics* **79**, 066503 (2016).
7. B. K. Greve, *et al.*, *Journal of the American Chemical Society* **132**, 15496 (2010).
8. B. H. Toby, R. B. Von Dreele, *Journal of Applied Crystallography* **46**, 544 (2013).

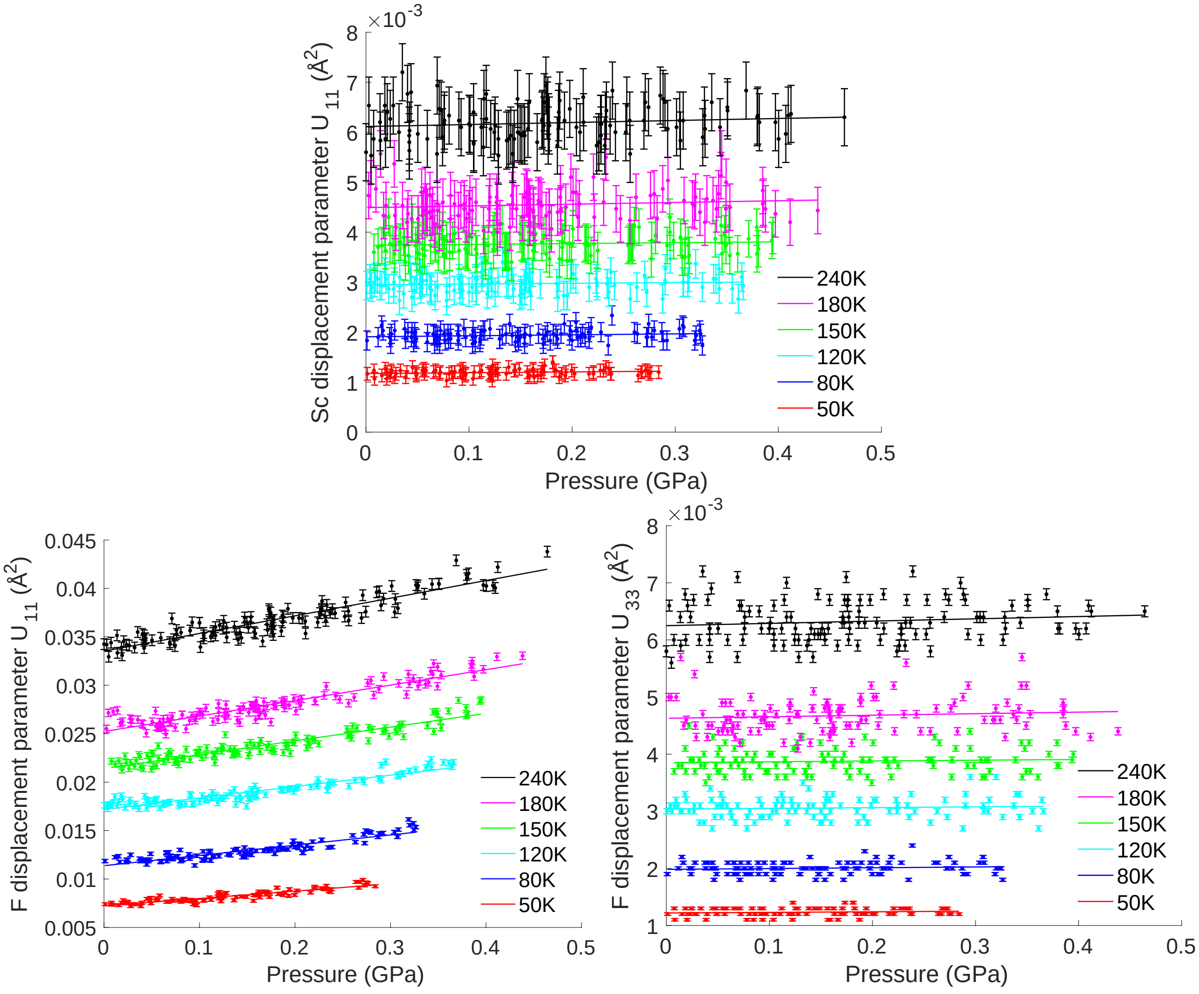


Figure S5: Variation of the Sc $U_{11}$ and F $U_{11}$ and $U_{33}$ with pressure at a small number of temperatures calculated by molecular dynamics simulation using the model described in the text.

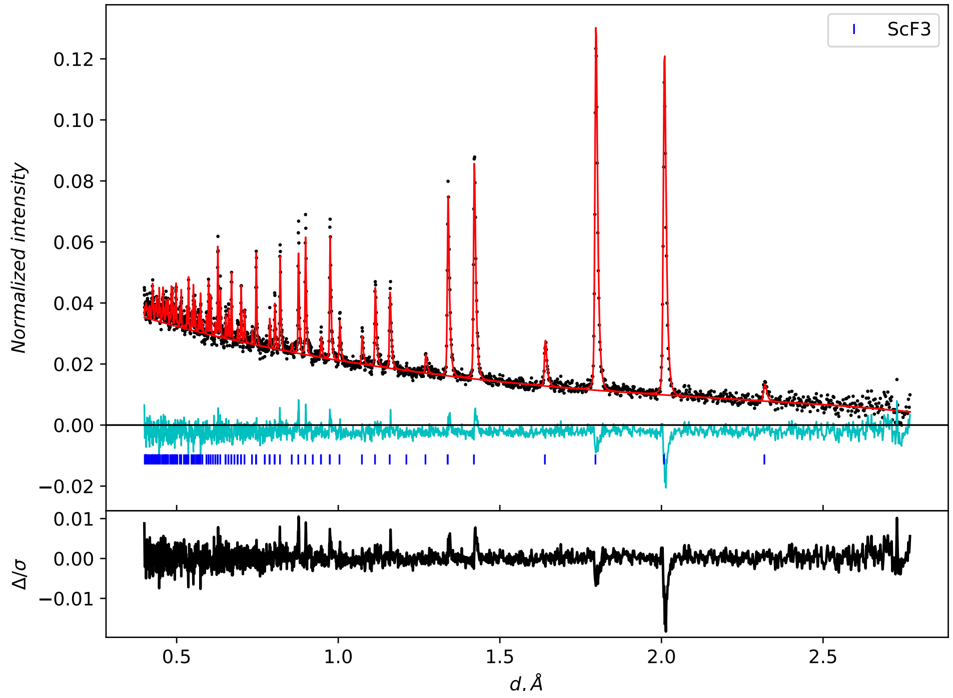


Figure S6: Diffraction data and fitted profile for $ScF_3$ at temperature of X K and pressure of X GPa calculated from the Rietveld refinement..

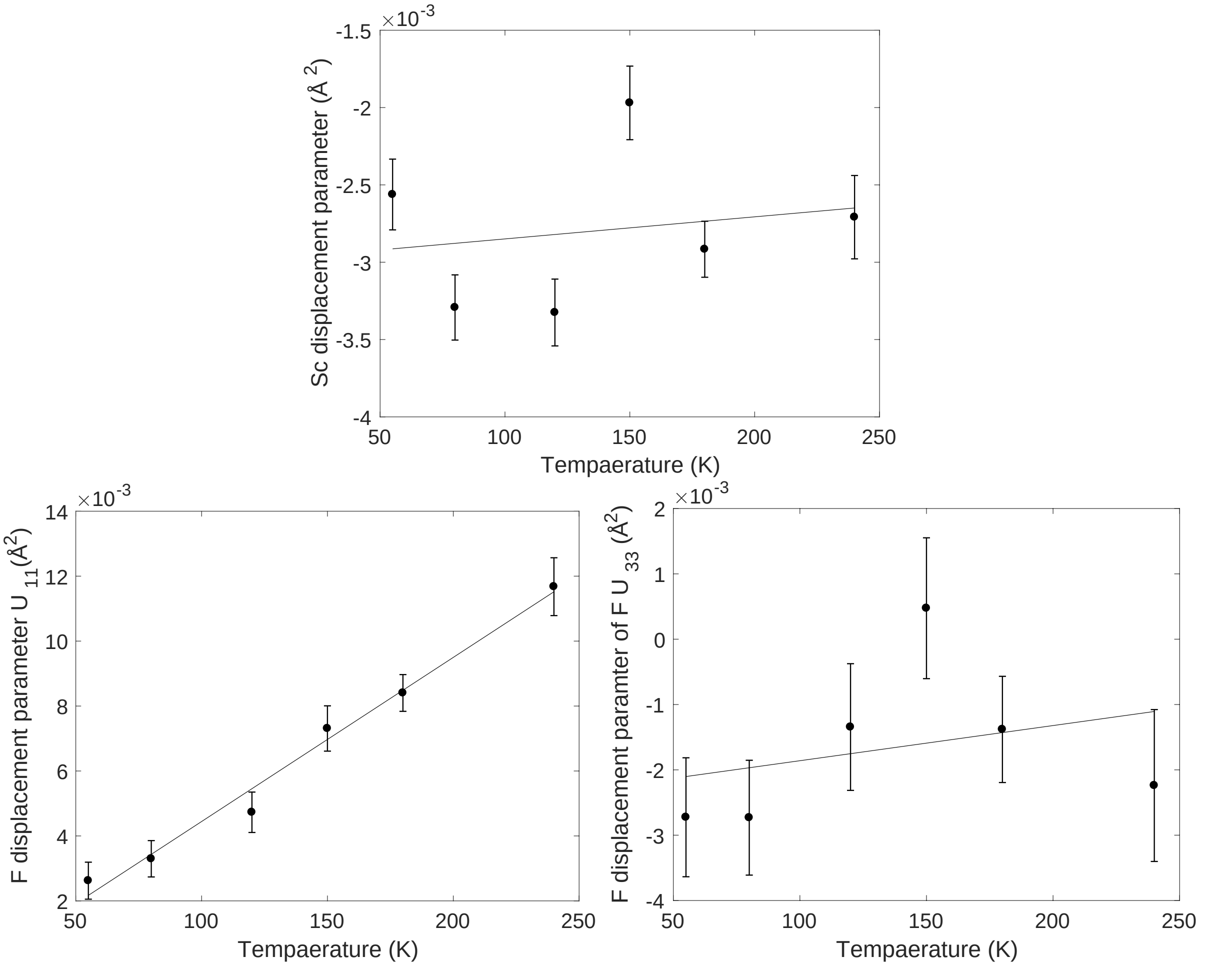


Figure S7: Variation of the Sc $U_{11}$ and F $U_{11}$ and $U_{33}$ with temperature at a small number of pressures obtained from the Rietveld refinement of experimental data.

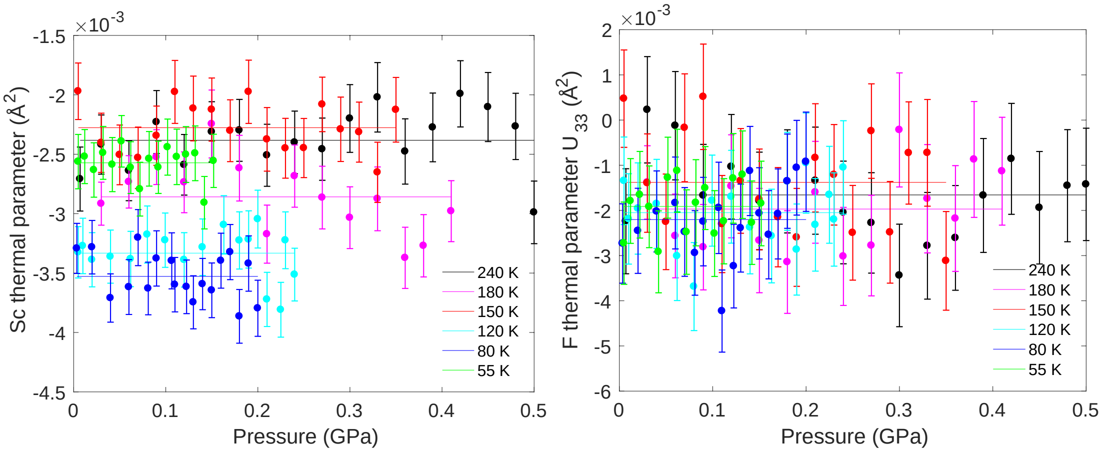


Figure S8: Variation of the Sc $U_{11}$ and F $U_{11}$ with pressure at a small number of temperatures obtained from the Rietveld refinement of experimental data.
